# Supplementary material for: Active Visual Localization for Multi-Agent Collaboration: A Data-Driven Approach
Source: arXiv:2310.02650 source file (2024-08-06)
Supplement: Supplementary file 1 [file appendix_datasheets.tex]

\chapter{Datasheets}\label{sec:datasheets}

\includepdf[scale=0.75]{images/datasheets.pdf}
