# Supplementary material for: Active Visual Localization for Multi-Agent Collaboration: A Data-Driven Approach
Source: arXiv:2310.02650 source file (2024-08-06)
Supplement: Supplementary file 2 [file appendix_text.tex]

\chapter{Irgendwas}\label{sec:irgendwas}

Bla bla \dots
